# Supplementary material for: Statehood Without Capacity
Source: arXiv:2604.11384 source file (2026-04-13)
Supplement: Supplementary file 1 [file appendix.tex]

\section{Visual vocabulary of an Elementary System Net}
\label{app:elsysnet}

\begin{figure}
    \includegraphics[scale=1]{graphics/visual_vocabulary_elementary_system_net}
    \caption{A circle depicts a place, a rectangle depicts a transition and an arrow depicts and arc. The arrow connects places with transitions and can be bent for that purpose. The green color is the standard color of the }
    \label{fig:visual_vocabulary_elementary_system_net}
\end{figure}
